# Supplementary material for: A strengthening on odd cycles in graphs of given chromatic number
Source: arXiv:2012.10624 ancillary file (2021-04-06)
Supplement: Supplementary file 1 [file Appendix.pdf]

# An appendix to “A strengthening on odd cycles in graphs of given chromatic number”

Jun Gao Qingyi Huo Jie Ma

School of Mathematical Sciences
University of Science and Technology of China
Hefei, Anhui, 230026, P.R. China.

## 1 Introduction

In this appendix, we prove the following results.

**Theorem 1.1.** *Every graph of chromatic number four contains two cycles of consecutive lengths the shortest one of which is odd.*

**Theorem 1.2.** *Every graph of chromatic number five contains three cycles of consecutive lengths the shortest one of which is odd.*

## 2 Preliminaries

We follow the notation in [2]. We need the following result on graphs containing a triangle in [2].

**Theorem 2.1** ( [2]). *Let $k \geq 2$ be an integer. Every 2-connected graph $G$ of minimum degree at least $k$ containing a triangle $K_3$ contains $k$ cycles of consecutive lengths, except that $G = K_{k+1}$.*

We say that $(G, x, y)$ is a *rooted graph* if $G$ is a graph and $x, y$ are two distinct vertices of $G$. The *minimum degree* of a rooted graph $(G, x, y)$ is $\min\{d_G(v) : v \in V(G) - \{x, y\}\}$. We also say that a rooted graph $(G, x, y)$ is 2*-connected* if $G + xy$ is 2-connected. We say that $k$ paths or $k$ cycles $P_1, P_2, \ldots, P_k$ are *admissible* if $|P_1| \geq 2$ and $|P_1|, |P_2|, \ldots, |P_k|$ form an arithmetic progression of length $k$ with common difference one or two.

We need the following result [1] on admissible paths between two vertices in a 2-connected rooted graph.

**Theorem 2.2** ( [1] Theorem 3.1). *Let $k$ be a positive integer. If $(G, x, y)$ is a 2-connected rooted graph of minimum degree at least $k + 1$, then there exist $k$ admissible paths from $x$ to $y$ in $G$.*

A cycle $C$ in a connected graph $G$ is *non-separating* if $G - V(C)$ is connected. We need the following lemma proved by Krusenstjerna-Hafstrøm and Toft [3]. [1]

**Theorem 2.3** ( [3] Lemma 4). *For any integer $k \geq 4$, every $k$-critical graph contains a non-separating induced odd cycle*

[1] We remark that the case $k = 4$ was explicitly stated and proved by Krusenstjerna-Hafstrøm and Toft [3, Theorem 4], but their proof works for every $k \geq 4$ as well.

# 3 Proof of Theorem 1.1

*Proof of Theorem 1.1.* It suffices to consider 4-critical graphs $G$. By Theorem 2.1, we may assume that $G$ is $K_3$-free. By Theorem 2.3, $G$ contains a non-separating induced odd cycle. We choose the non-separating induced odd cycle $C := v_0v_1 \dots v_{2\ell}v_0$ such that $|V(C)|$ is minimum, where the indices are taken under the additive group $\mathbb{Z}_{2\ell+1}$. Since $G$ is $K_3$-free, we have that $\ell \geq 2$. Let $H := G - V(C)$.

Suppose that there exists a non-cut-vertex $x$ of $H$ which has at least two neighbors on $C$. Since $C$ is an odd cycle, there exist two distinct vertices $v_i, v_j$ in $N_C(x)$ such that the odd path between $v_i$ and $v_j$ on $C$ has no internal vertices in $N_C(x)$. Let $Q_o$ and $Q_e$ be the odd and even path between $v_i$ and $v_j$ in $C$, respectively. Since $G$ is $K_3$-free, we have that $|E(Q_o)| > 1$. Let $C' := xv_i \cup Q_o \cup v_jx$. Note that $C'$ is an induced odd cycle. Suppose that $N_H(Q_e - \{v_i, v_j\}) - x = \emptyset$. Since $G$ has minimum degree at least 3 and $C$ is an induced cycle, we have that $x$ is adjacent every vertex in $Q_e - \{v_i, v_j\}$. It follows that $G$ contains a $K_3$, a contradiction. Therefore there is a vertex in $Q_e - \{v_i, v_j\}$ which has a neighbor in $H - x$. Hence, $C'$ is a non-separating induced odd cycle. By the minimality of $C$, we have that $|V(C')| \geq |V(C)|$ which implies that $|E(Q_e)| = 2$. Without loss of generality, we may assume that $j = i + 2$. Let $y$ be one neighbor of $v_{i+\ell+1}$ in $H$. Let $Q$ be a fixed path between $x$ and $y$ in $H$. Since $\ell \geq 2$, $C_{i+2,i+\ell+1} \cup v_{i+\ell+1}y \cup Q \cup xv_{i+2}$, $C_{i+\ell+1,i} \cup v_{i+\ell+1}y \cup Q \cup xv_i$, $C_{i,i+\ell+1} \cup v_{i+\ell+1}y \cup Q \cup xv_i$, $C_{i+\ell+1,i+2} \cup v_{i+\ell+1}y \cup Q \cup xv_{i+2}$ are 4 cycles of consecutive lengths. Therefore every non-cut-vertex of $H$ has at most one neighbor on $C$.

Suppose that $H$ is non-bipartite. Assume that $H$ is 2-connected. Let $w_1$ be the neighbor of $v_0$ in $H$. Since $w_1$ is a non-cut-vertex of $H$, $N_C(w_1) = \{v_0\}$. Note that $G$ has minimum degree at least 3. We have that $v_\ell$ has a neighbor $w_2 \neq w_1$ in $H$. Since $H$ is 2-connected and non-bipartite, there are two paths $Q_1, Q_2$ from $w_1$ to $w_2$ in $H$ with different parity. Then two of $v_0w_1 \cup Q_i \cup w_2v_\ell \cup C_{0,\ell}$, $v_0w_1 \cup Q_i \cup w_2v_\ell \cup C_{\ell,0}$, where $i = 1, 2$, are desired cycles of consecutive lengths. Therefore $H$ is not 2-connected. Let $B$ be a non-bipartite block of $H$. Let $c \in B$ be a cut-vertex of $H$. Let $D_1$ be the component of $H - c$ containing $B$ and let $D_2 = H - D_1$. Since $G$ is 2-connected and has minimum degree at least 3 and $C$ is an induced odd cycle, there exist $v_i, v_{i+\ell}$ such that $v_i$ has a neighbor $w_3$ in $D_1$ and $v_{i+\ell}$ has a neighbor $w_4$ in $D_2$. Using the block structure of $D_1$, there exist two paths $Q'_1, Q'_2$ from $c$ to $w_3$ in $G[D \cup \{c\}]$ with different parity. Let $L$ be a fixed path from $w_4$ to $c$ in $D_2$. Then two of $v_iw_3 \cup Q'_j \cup L \cup w_4v_{i+\ell} \cup C_{i,i+\ell}$, $v_iw_3 \cup Q'_j \cup L \cup w_3v_{i+\ell} \cup C_{i+\ell,i}$, where $j \in [2]$, are desired cycles of consecutive lengths.

Therefore $H$ is bipartite and let $(X, Y)$ be the bipartition of $H$. For a vertex $v \in V(C)$, we say it is of *type-X* if it has a neighbor in $X$ and it is of *type-Y* if it has a neighbor in $Y$. [2]

Assume that $|V(C)| \equiv 3$ modulo 4. Note that $\ell$ is odd. Suppose that there exist two consecutive vertices of $C$ such that they are of different types. Without loss of generality, we may assume that $v_0, v_1$ are of different types. Then $v_{\ell+1}$ must be of the same type of one of $\{v_0, v_1\}$. Without loss of generality, we may assume that $v_0, v_{\ell+1}$ are of type-$X$. Let $x_1$ be one neighbor of $v_0$ in $X$ and $x_2$ be one neighbor of $v_{\ell+1}$ in $X$. Note that there is an even path $P_e$ from $x_1$ to $x_2$ in $H$. Then $C_{\ell+1,0} \cup P_e \cup v_0x_1 \cup v_{\ell+1}x_2$, $C_{0,\ell+1} \cup P_e \cup v_0x_1 \cup v_{\ell+1}x_2$ are two desired cycles of consecutive lengths. Therefore, all vertices of $C$ are of the same type. Similarly, we could obtain two desired cycles of consecutive lengths.

Therefore $|V(C)| \equiv 1$ modulo 4. Note that $\ell$ is even. Without loss of generality, we may assume that $v_0$ is of type-$X$ and let $x_3$ be a neighbor of $v_0$ in $X$. If $v_\ell$ is of type-$Y$ and let $y_1$ be a neighbor of $v_\ell$ in $Y$, then there exists an odd path $P_o$ from $x_3$ to $y_1$ in $H$. Then $C_{0,\ell} \cup P_o \cup v_0x_3 \cup v_\ell y_1$, $C_{\ell,0} \cup P_o \cup v_0x_3 \cup v_\ell y_1$ are two desired cycles of consecutive lengths. Therefore $v_\ell$ can only be of type-$X$. Note that $\ell$ is a generator of the additive group $\mathbb{Z}_{2\ell+1}$. So all vertices of $C$ can only be of type-$X$, that is, $N_H(C) \subseteq X$.

[2]We remark that a vertex can be both of type-$X$ and type-$Y$.

Suppose that every vertex of $H$ has at most one neighbor on $C$. Since $C$ is an induced odd cycle, we could properly color vertices of $C$ with colors $1, 2$ and 3. For a vertex $x \in X$, if $x$ has neighbor on $C$ with color 1 or 2, then we color $x$ with color 3. Next, we color remaining vertices of $X$ with color 1 and color vertices of $Y$ with color 2. It is obvious that this is a proper 3-coloring of $G$, a contradiction.

Therefore there exists a vertex in $X$ which has at least two neighbors on $C$. Since every non-cut-vertex of $H$ has at most one neighbor on $C$, we have that $H$ is not 2-connected. Let $Z$ be the set of cut-vertices of $H$ which have at least two neighbors on $C$. Note that $Z \subseteq X$.

Suppose that there exists a vertex $v \in V(C)$ such that $N_Z(v) = \emptyset$. We define a coloring of $G$ according to the rule below: (i) color $v$ with color 3 and color $V(C) - v$ alternately with colors 1 and 2, (ii) color vertices in $N_X(v)$ with color 1, (iii) color vertices in $X - N(v)$ with color 3, (iv) color vertices in $Y$ with color 2. Note that every vertex in $N_X(v)$ has exactly one neighbor on $C$. It is not hard to check that this is a proper 3-coloring of $G$, a contradiction.

Therefore any vertex of $C$ has a neighbor in $Z$. Let $z \in Z$ such that $Z - \{z\}$ is contained in a component of $H - z$. Choose $v_i, v_j \in N_C(z)$ such that the length of even path between $v_i$ and $v_j$ in $C$ is as short as possible. Let $Q_o, Q_e$ be the odd and even paths between $v_i$ and $v_j$ in $C$ respectively. Let $2p + 1$ denote the length of $Q_o$. Without loss of generality, we may assume that $j = i + 2p + 1$.

Assume that $|E(Q_o)| \equiv 3$ modulo 4. So $p$ is odd. Since $G$ is $K_3$-free, at least one of $v_{i+p}, v_{i+p+1}$ has a neighbor in $Z - z$. Without loss of generality, we may assume that $v_{i+p}$ has a neighbor in $z' \in Z - z$. Let $R$ be a fixed path between $z$ and $z'$ in $H$. Note that $R$ has even length. So $zv_i \cup C_{i,i+p} \cup v_{i+p}z' \cup R$, $zv_{i+2p+1} \cup C_{i+p,i+2p+1} \cup v_{i+p}z' \cup R$ are two desired cycles of consecutive lengths.

Therefore $|E(Q_o)| \equiv 1$ modulo 4. So $p$ is even. Since $G$ is $K_3$-free, we have $p \geq 2$. Let $|E(Q_e)| = 2q$. Since $|V(C)| \equiv 1$ modulo 4, we have that $q$ is even. Since $G$ is $K_3$-free, at least one of $v_{i+p}, v_{i+p+1}$ has a neighbor in $Z - z$. Without loss of generality, $v_{i+p}$ has a neighbor in $z_1 \in Z$. Let $z_2 \in Z$ be the neighbor of $v_{j+q}$. Suppose that $z_2 \neq z$. By the choice of $z$, we could find a path $R'$ between $z_1$ and $z_2$ in $H$. Note that $R'$ has even length. Then cycles $C_{i-q,i+p} \cup v_{i+p}z_1 \cup R' \cup v_{i-q}z_2$, $C_{i+p,i-q} \cup v_{i+p}z_1 \cup R' \cup v_{i-q}z_2$, $C_{i,i+p} \cup v_i z v_j \cup C_{j,j+q} \cup R' \cup z_1 v_{i+p} \cup v_{i-q}z_2$ have lengths $p+q+2+|E(R')|$, $p+q+3+|E(R')|$, $p+q+4+|E(R')|$, respectively. Therefore $z_2 = z$, that is $v_{i-q} \in N_C(z)$. It follows that the even path between $v_i$ and $v_{i-q}$ is shorter, a contradiction. ∎

## 4 Basic lemmas

In the rest of the paper, we consider graphs of chromatic number five. In view of Theorem 2.1, we may assume that all graphs considered in the rest of the paper are $K_3$-free.

Let $C$ be a cycle with vertices $v_0, v_1, \ldots, v_{t-1}$ in cyclic order. Let $C_{i,j}$ denote the subpath $v_i v_{i+1} \ldots v_j$ of $C$, where the indices are taken under the additive group $\mathbb{Z}_t$. Let us first prove a few lemmas.

**Lemma 4.1.** *Let $G$ be a 2-connected graph. Assume that $G$ contains a non-separating induced cycle $C := v_0 v_1 \ldots v_{t-1} v_0$, where the indices are taken under the additive group $\mathbb{Z}_t$, such that every vertex of $C$ has a neighbor in $H := G - V(C)$ and $H$ is not 2-connected. Let $b$ be a cut-vertex of $H$ and $F$ be any component of $H - b$. If $s$ is a generator of the additive group $\mathbb{Z}_t$, then there exist two vertices $v_i, v_{i+s}$ such that $v_i$ has a neighbor in $F$ and $v_{i+s}$ has a neighbor in $H - F \cup \{b\}$.*

*Proof.* Suppose to the contrary that there are no $v_i$ and $v_{i+s}$ such that $v_i$ has a neighbor in $F$ and $v_{i+s}$ has a neighbor in $H - F \cup \{b\}$. Since $G$ is 2-connected, we have that $N_H(V(C)) \cap V(F) \neq \emptyset$. Without lose of generality, we may assume that $v_0$ has a neighbor in $F$. Then $N_H(v_s) \subseteq V(F) \cup \{b\}$. Since $s$ is a generator of the additive group $\mathbb{Z}_t$, we have that $N_H(V(C)) \subseteq V(F) \cup \{b\}$. It follows that $b$ is a cut-vertex of $G$, a contradiction. This completes the proof of the lemma. ∎

**Lemma 4.2.** *Let $G$ be a graph and let $C := v_0v_1\dots v_{2\ell}v_0$ be an odd cycle of length at least five, where the indices are taken under the additive group $\mathbb{Z}_{2\ell+1}$ for some $\ell \geq 2$. Suppose that there exists $z \in V(G) - V(C)$ such that $z$ is adjacent to $v_i$ and $v_{i+2}$ for some $i \in \mathbb{Z}_{2\ell+1}$. If there exists a path $L$ from $v_{i+\ell+1}$ to $z$ internally disjoint from $V(C)$, then $G$ contains four cycles of consecutive lengths.*

*Proof.* $C_{i+2,i+\ell+1} \cup L \cup zv_{i+2}$, $C_{i+\ell+1,i} \cup L \cup zv_i$, $C_{i,i+\ell+1} \cup L \cup zv_i$, $C_{i+\ell+1,i+2} \cup L \cup zv_{i+2}$ are 4 cycles of consecutive lengths in $G$. ∎

**Lemma 4.3.** *Let $C := v_0v_1\dots v_{t-1}v_0$ be a cycle of length at least five, where the indices are taken under the additive group $\mathbb{Z}_t$. For any two non-consecutive vertices $v_i, v_j$ on $C$, there exist two distinct vertices $v_p, v_q \in V(C) - \{v_i, v_j\}$, where $v_i, v_p, v_j, v_q$ in a cyclic order on $C$, such that $(|C_{i,p}| + |C_{j,q}|) - (|C_{q,i}| + |C_{p,j}|) = 1 + \epsilon$, where $\epsilon = 0$ if $t$ is odd and $\epsilon = 1$ if $t$ is even.*

*Proof.* Suppose that $C$ is odd. Without loss of generality, we may assume that $|C_{i,j}| = 2x + 1$ is odd and $|C_{j,i}| = 2y$ is even. Since $v_i, v_j$ are not adjacent in $C$, we have that $x \geq 1$. It follows that $v_{i+x+1} \neq v_j$. We have that $|C_{i,i+x+1}| = x + 1, |C_{i+x+1,j}| = x, |C_{j,j+y}| = y, |C_{j+y,i}| = y$, that is $(|C_{i,i+x+1}| + |C_{j,j+y}|) - (|C_{i+x+1,j}| + |C_{j+y,i}|) = 1$.

Therefore, $C$ is even. It follows $C_{i,j}$ and $C_{j,i}$ have the same parity. Assume that $|C_{i,j}| = 2m+1$ and $|C_{j,i}| = 2n + 1$. Since $v_i, v_j$ are not adjacent in $C$, we have that $m, n \geq 1$. It follows that $v_{i+m+1} \neq v_i$ and $v_{j+n+1} \neq v_j$. We have that $|C_{i,i+m+1}| = m + 1, |C_{i+m+1,j}| = m, |C_{j,j+n+1}| = n + 1, |C_{j+n+1,i}|| = n$, that is $(|C_{i,i+m+1}|| + |C_{j,j+n+1}|) - (|C_{i+m+1,j}| + |C_{j+n+1,i}|) = 2$. Therefore, $|C_{i,v_j}| = 2k$ and $|C_{j,i}| = 2l$. Since $C$ has length at least 5, at least one of $k, \ell$ is at least 2. Without loss of generality, we may assume that $k \geq 2$. It follows that $v_{i+k+1} \neq v_i$. We have that $|C_{i,i+k+1}| = k + 1, |C_{i+k+1,j}| = k - 1, |C_{j,j+\ell}| = \ell, |C_{j+\ell,i}| = \ell$, that is $(|C_{i+k+1,j}|| + |C_{j,j+\ell}|) - (|C_{i+k+1,j}| + |C_{j+\ell,j}|) = 2$. ∎

**Lemma 4.4.** *Let $G$ be a 2-connected $K_3$-free graph consisted of $C, C'$ and $H$ satisfying the followings:*

1. *$C$ is an induced odd cycle and every vertex of $C$ has degree at least four in $G$,*
2. *$C'$ is an induced cycle and every vertex of $C'$ has at most one neighbor on $C$,*
3. *$H$ is connected and every vertex of $C'$ has at least one neighbor in $H$.*

*If one of the following conditions is true,*

1. *$C'$ is even and $N_G(C) \subseteq V(C')$.*
2. *$C'$ is even, $N_H(C) \neq \emptyset$ and some vertex of $C$ has at least one neighbor on $C'$.*
3. *$C'$ is odd, $N_H(C) \neq \emptyset$ and some vertex of $C$ has at least two neighbors on $C'$.*

*Then $G$ contains four cycles of consecutive lengths.*

*Proof.* Let $C := v_0v_1\dots v_{2\ell}v_0$, where $\ell \geq 2$ be an induced odd cycle of $G$, where the indices are taken under the additive group $\mathbb{Z}_{2\ell+1}$. Assume that $C' := u_0u_1\dots u_{2h_e-1}u_0$ where $h_e \geq 2$, is an induced even cycle of $G$, where the indices are taken under the additive group $\mathbb{Z}_{2h_e}$.

Suppose that $N_G(C) \subseteq V(C')$. Let $u_i$ be the neighbor of $v_0$. Since every vertex in $C'$ has at most one neighbor in $C$ and every vertex on $C$ has at least two neighbors on $C'$, we have that $|V(C')| \geq 2|V(C)| \geq 10$ and at least one of $v_\ell, v_{\ell+1}$ has a neighbor $u_j \in V(C') - \{u_{i-1}, u_i, u_{i+1}\}$. Without loss of generality, we assume that $v_\ell$ is adjacent to $u_j$. By Lemma 4.3, there exist two vertices $u_p, u_q$ in $V(C') - \{u_i, u_j\}$ such that $(|C'_{i,p}| + |C'_{j,q}|) - (|C'_{q,i}| + |C'_{p,j}|) = 2$. Since $H$ is connected and every vertex of $C'$ has at least one neighbor in $H$. There exists a path $L$ between $v_p$ and $v_q$ internally disjoint from

$V(C)\cup V(C')$. Then $C_{0,\ell}\cup v_0u_i\cup C'_{q,i}\cup C'_{p,j}\cup v_\ell u_j\cup L$, $C_{\ell,0}\cup v_0u_i\cup C'_{q,i}\cup C'_{p,j}\cup v_\ell u_j\cup L$, $C_{0,\ell}\cup v_0u_i\cup C'_{i,p}\cup C'_{j,q}\cup v_\ell u_j\cup L$, $C_{\ell,0}\cup v_0u_i\cup C'_{i,p}\cup C'_{j,q}\cup v_\ell u_j\cup L$ are 4 cycles of consecutive lengths in $G$.

Suppose that $N_H(C)\neq\emptyset$ and $N_G(C)\cap V(C')\neq\emptyset$, without loss of generality, we may assume that $u_j$ and $v_i$ are adjacent in $G$. Suppose that $v_{i+\ell}$ has a neighbor $z$ in $H$. Let $w$ be the neighbor of $u_{j+h_e-1}$ in $H$. Let $M$ be a fixed path between $z$ and $w$ in $H$. Then $C_{i,i+\ell}\cup v_iu_j\cup v_{i+\ell}z\cup M\cup wu_{j+h_e-1}\cup C'_{j,j+h_e-1}$, $C_{i+\ell,i}\cup v_iu_j\cup v_{i+\ell}z\cup M\cup wu_{j+h_e-1}\cup C'_{j,j+h-1}$, $C_{i,i+\ell}\cup v_iu_j\cup v_{i+\ell}z\cup M\cup wu_{j+h_e-1}\cup C'_{j+h_e-1,j}$, $C_{i+\ell,i}\cup v_iu_j\cup v_{i+\ell}z\cup M\cup wu_{j+h_e-1}\cup C'_{j+h_e-1,j}$ are 4 cycles of consecutive lengths in $G$. Therefore $N_G(v_{i+\ell})\subseteq V(C')$. Since $\ell$ is the generator of the additive group $\mathbb{Z}_{2\ell+1}$, we have that $N_G(C)\subseteq V(C')$, a contradiction.

Now, we assume that $C':=u_0u_1\dots u_{2h_o}u_0$ where $h_o\geq 2$, is an induced odd cycle of $G$, where the indices are taken under the additive group $\mathbb{Z}_{2h_o+1}$. Without loss of generality, we may assume that $v_0$ has two neighbors $u_\alpha,u_\beta$ on $C'$. Assume that the even path between $u_\alpha$ and $u_\beta$ in $C'$ has length $2r$, that is $\beta=\alpha+2r$, where $r\geq 1$. Let $w'$ be the neighbor of $u_{\alpha+r-1}$ in $H$. If $v_\ell$ has a neighbor $z'$ in $H$, then there exists a path $N$ between $z'$ and $w'$ in $H$. It follows that $C_{0,\ell}\cup v_0u_\alpha\cup C'_{\alpha,\alpha+r-1}\cup u_{\alpha+r-1}w'\cup N\cup z'v_\ell$, $C_{\ell,0}\cup v_0u_\alpha\cup C'_{\alpha,\alpha+r-1}\cup u_{\alpha+r-1}w'\cup N\cup z'v_\ell$, $C_{0,\ell}\cup v_0u_\beta\cup C'_{\alpha+r-1,\beta}\cup u_{\alpha+r-1}w'\cup N\cup z'v_\ell$, $C_{\ell,0}\cup v_0u_\beta\cup C'_{\alpha+r-1,\beta}\cup u_{\alpha+r-1}w'\cup N\cup z'v_\ell$ are 4 cycles of consecutive lengths in $G$. Therefore $N_G(v_\ell)\subseteq V(C')$. Since every vertex of $C$ has degree at least 4 in $G$ and $C$ is an induced odd cycle, we have that $N_G(C)\subseteq V(C')$, a contradiction. ∎

**Lemma 4.5.** *Let $G$ be a 2-connected graph consisted of $C$ and $H$ satisfying the followings:*

1. *$C$ is an induced odd cycle and every vertex of $C$ has at least one neighbor in $H$,*
2. *$H$ is connected but is not 2-connected and every non-cut-vertex of $H$ has degree at least three in $H$.*

*Let $B_1,\dots,B_s$ be all end-blocks of $H$ with cut-vertices $b_1,\dots,b_s$ respectively. Then either*

1. *$G$ contains three cycles of lengths $2m+1,2m+2,2m+3$ for some integer $m$, or*
2. *there exists a vertex $v$ on $C$ such that $N_C(\cup_{i\in[s]}(B_i-b_i))=\{v\}$ and two admissible paths with difference one from $b_i$ to $v$ in $G[B_i\cup\{v\}]$.*

*Proof.* Let $C:=v_0v_1\dots v_{2\ell}v_0$ be an induced odd cycle of $G$, where the indices are taken under the additive group $\mathbb{Z}_{2\ell+1}$. Since $C$ is odd and $G$ is 2-connected, by Lemma 4.1, there exist $v_{p_i},v_{p_i+\ell}$ such that $v_{p_i}$ has a neighbor $z_i$ in $B_i-b_i$ and $v_{p_i+\ell}$ has a neighbor $w_i$ in $H-(B_i-b_i)$ for each $i\in[s]$. Since every non-cut-vertex of $H$ has degree at least 3 in $H$, we have that $B_i$ is 2-connected, that is $(B_i,z_i,b_i)$ is 2-connected of minimum degree at least 3. By Theorem 2.2, there are 2 admissible paths $Q_{i,1},Q_{i,2}$ between $z_i$ and $b_i$ in $B_i$. Let $L_i$ be a fixed path between $b_i$ and $w_i$ in $H-(B_i-b_i)$. If $|E(Q_{i,1})|-|E(Q_{i,2})|=2$, then $C_{p_i,p_i+\ell}\cup v_{p_i}z_i\cup Q_{i,2}\cup L_i\cup w_iv_{p_i+\ell}$, $C_{p_i+\ell,p_i}\cup v_{p_i}z_i\cup Q_{i,2}\cup L_i\cup w_iv_{p_i+\ell}$, $C_{p_i,p_i+\ell}\cup v_{p_i}z_i\cup Q_{i,1}\cup L_i\cup w_iv_{p_i+\ell}$, $C_{p_i+\ell,p_i}\cup v_{p_i}z_i\cup Q_{i,1}\cup L_i\cup w_iv_{p_i+\ell}$ are 4 cycles of consecutive lengths in $G$. Hence $|E(Q_{i,1})|-|E(Q_{i,2})|=1$.

For any vertex $v_q\neq v_{p_i}$ on $C$, suppose that $v_q$ has a neighbor $u$ in $B_j-b_j$ for some $j\neq i$. Note that $(B_j,u,b_j)$ is 2-connected of minimum degree at least 3. By Theorem 2.2, there are 2 admissible paths $R_1,R_2$ between $u$ and $b_j$ in $B_j$. Let $L$ be a fixed path between $b_i$ and $b_j$ in $H-(B_i-b_i)\cup(B_j-b_j)$. If $|E(R_1)|-|E(R_2)|=2$, then $Q_{i,2}\cup L\cup R_2\cup uv_q\cup C_{q,p_i}\cup v_{p_i}z$, $Q_{i,1}\cup L\cup R_2\cup uv_q\cup C_{q,p_i}\cup v_{p_i}z$, $Q_{i,2}\cup L\cup R_1\cup uv_q\cup C_{q,p_i}\cup v_{p_i}z$, $Q_{i,1}\cup L\cup R_1\cup uv_q\cup C_{q,p_i}\cup v_{p_i}z$ are 4 cycles of consecutive lengths in $G$. Therefore $|E(R_1)|-|E(R_2)|=1$. Then $Q_{i,\alpha}\cup L\cup R_\beta\cup uv_q\cup C_{q,p_i}\cup v_pz$ are 3 cycles of consecutive lengths in $G$ and $Q_{i,\alpha}\cup L\cup R_\beta\cup uv_q\cup C_{p_i,q}\cup v_pz$ are 3 cycles of consecutive lengths in $G$, where $\alpha,\beta=1,2$. Since $|C_{p_i,q}|$ and $|C_{q,p_i}|$ are of different parity, one of above two classes are three cycles of desired lengths.

Therefore, $N_H(v_q) \cap (\cup_{j\in[s]-\{i\}}(B_j - b_j)) = \emptyset$. Since $G$ is 2-connected, $N_C(B_j - b_j) \neq \emptyset$ for any $j \neq i$. This forces that $N_C(B_j - b_j) = \{v_{p_i}\}$ for any $j \neq i$. By symmetry, we have that $N_C(B_i - b_i) = \{v_{p_i}\}$. This completes the proof of Lemma 4.5. ∎

**Lemma 4.6.** *Let $G$ be a 2-connected $K_3$-free graph consisted of $C, C'$ and $H$ satisfying the followings:*

1. *$C$ is an induced odd cycle and $N_G(C) \subseteq V(C')$,*
2. *$C'$ is an induced odd cycle and every vertex of $C'$ has at least one neighbor in $H$,*
3. *$H$ is connected and every non-cut-vertex of $H$ has at most one neighbor on $C'$*
4. *$G[C' \cup H]$ is 2-connected and every vertex of $G[C' \cup H]$ has at most one neighbor on $C$.*

*If every vertex in $V(C) \cup V(H)$ has degree at least four in $G$, then $G$ contains three cycles of lengths $2m+1, 2m+2, 2m+3$ for some integer $m$.*

*Proof.* Let $C := v_0v_1 \dots v_{2\ell}v_0$ be an induced odd cycle of $G$, where the indices are taken under the additive group $\mathbb{Z}_{2\ell+1}$. Let $C' := u_0u_1 \dots u_{2h}u_0$ where $h \geq 2$, be an induced odd cycle of $G$, where the indices are taken under the additive group $\mathbb{Z}_{2h+1}$. Let $u_i$ be the neighbor of $v_0$. Since every vertex in $C'$ have at most one neighbor on $C$ and every vertex in $C$ has at least two neighbors on $C'$, we have that $|V(C')| \geq 2|V(C)| \geq 10$ and at least one of $v_\ell, v_{\ell+1}$ has a neighbor $u_j \in V(C') - \{u_{i-1}, u_i, u_{i+1}\}$. Without loss of generality, we assume that $v_\ell$ is adjacent to $u_j$. By Lemma 4.3, there exist two vertices $u_p, u_q$ in $V(C') - \{u_i, u_j\}$ such that $(|C'_{i,p}| + |C'_{j,q}|) - (|C'_{q,i}| + |C'_{p,j}|) = 1$. Let $z_p, z_q$ be the neighbors of $u_p, u_q$ in $H$ respectively. Note that there are two pairs of vertices satisfying the conclusion of Lemma 4.3. Since $G$ is $K_3$-free, we may assume that $z_p \neq z_q$. Assume that $H$ is 2-connected. Since $N_G(C) \subseteq V(C')$ and every non-cut-vertex of $H$ has at most one neighbor on $C'$. We have that $(H, z_p, z_q)$ is 2-connected of minimum degree at least 3. By Theorem 2.2, there exist two admissible paths $P_1, P_2$ between $z_p$ and $z_q$ in $H$. Then there are at least 4 cycles of consecutive lengths in $G$ in $C_{0,\ell} \cup v_0u_i \cup C'_{q,i} \cup C'_{p,j} \cup v_\ell u_j \cup u_qz_q \cup P_\gamma \cup u_pz_p$, $C_{\ell,0} \cup v_0u_i \cup C'_{q,i} \cup C'_{p,j} \cup v_\ell u_j \cup u_qz_q \cup P_\gamma \cup u_pz_p$, $C_{0,\ell} \cup v_0u_i \cup C'_{i,p} \cup C'_{j,q} \cup v_\ell u_j \cup u_qz_q \cup P_\gamma \cup u_pz_p$, $C_{\ell,0} \cup v_0u_i \cup C'_{i,p} \cup C'_{j,q} \cup v_\ell u_j \cup u_qz_q \cup P_\gamma \cup u_pz_p$, where $\gamma = 1, 2$.

Therefore $H$ is not 2-connected. Let $B_1, \dots, B_s$ be all end-blocks of $H$ with cut-vertices $b_1, \dots, b_s$ respectively. Since every non-cut-vertex of $H$ has degree at least 3 in $H$, we have that $B_i$ is 2-connected for $i \in [s]$. Note that $C'$ is odd. Using Lemma 4.5 for $G[H \cup C']$, there exists an vertex $u_d$ on $C'$ such that for every $i \in [s]$, $N_{C'}(B_i - b_i) = \{u_d\}$ and there exist two paths $Q_{i,1}, Q_{i,2}$ from $u_i$ to $u_d$ in $G[B_i \cup \{u_d\}]$ satisfying $|E(Q_{i,1})| - |E(Q_{i,2})| = 1$. Note that vertices in $H$ have no neighbors on $C$. It follows that every vertex in $H$ has degree at least 4 in $G[C' \cup H]$. Since every vertex in $B_1 - b_1$ has degree at least 4, we have that $(G[B_1 \cup \{u_d\}], b_1, u_d)$ is 2-connected of minimum degree at least 4. By Theorem 2.2, there exist three admissible paths $R_1, R_2, R_3$ between $b_1$ and $u_d$ in $G[B_1 \cup \{u_d\}]$. Let $L$ be a fixed path between $b_1$ and $b_2$ in $H - (B_1 - b_1) \cup (B_2 - b_2)$. Then there are at least 4 cycles of consecutive lengths in $G$ in $Q_{2,\alpha} \cup L \cup R_\beta$ , where $\alpha = 1, 2$ and $\beta = 1, 2, 3$. ∎

## 5 The key lemma

In this section, we show that none of three cycles of consecutive lengths which start with an odd number implies that the graph has a specific structure.

**Lemma 5.1.** *Let $G$ be a 2-connected $K_3$-free graph of minimum degree at least four. Suppose that $G$ contains a non-separating induced odd cycle $C$ such that $H := G - V(C)$ is 2-connected and every vertex*

*of $H$ has at most one neighbor on $C$. If $H$ contains a non-separating induced cycle $C'$ such that every non-cut-vertex of $H' := H - V(C')$ has at most one neighbor on $C'$ unless $C'$ is a cycle of length four, then either*

1. *$G$ contains three cycles of lengths $2m+1, 2m+2, 2m+3$ for some integer $m$, or*
2. *$C$ and $C'$ have following properties: (i) $C'$ is odd , (ii) there is no edge between $C$ and $C'$, (iii) $H'$ is 2-connected and any vertex of $H'$ has at most one neighbor in $V(C) \cup V(C')$ in $G$.*

*Proof.*

**Claim 1.** *$C'$ is odd.*

*Proof.* Suppose to the contrary that $C' := u_0u_1 \dots u_{2h-1}u_0$ is an even cycle, where the indices are taken under the additive group $\mathbb{Z}_{2h}$. By Lemma 4.4, we know that $N_G(C) \cap V(C') = \emptyset$, that is $N_G(C) \subseteq V(H')$.

Assume that $H'$ is 2-connected. Let $z$ be the neighbor of $v_0$ in $H'$. Since every vertex in $H'$ has at most one neighbor on $C$, $v_\ell$ has a neighbor $z' \neq z$ in $H'$. Let $w$ be the neighbor of $u_0$ in $H'$. We will show that $u_{h-1}$ contains a neighbor $w' \neq w$ in $H'$. Suppose that $C'$ is a cycle of length 4. Then $u_1$ has a neighbor $w' \neq w$ in $H'$, since $G$ does not contain a $K_3$ subgtaph. Therefore $C'$ is not of length 4. Since every non-cut-vertex of $H'$ has at most one neighbor on $C'$, $u_{h-1}$ contains a neighbor $w' \neq w$ in $H'$. Note that $H'$ is 2-connected. There exist two disjoint paths $Q_1, Q_2$ between $\{z, z'\}$ and $\{w, w'\}$ in $H'$. Without loss of generality, we may assume that $Q_1$ links $z$ and $w$ and $Q_2$ links $z'$ and $w'$. Then $C_{0,\ell} \cup v_0z \cup Q_1 \cup wu_0 \cup C'_{0,h-1} \cup u_{h-1}w' \cup Q_2 \cup z'v_\ell$, $C_{\ell,0} \cup v_0z \cup Q_1 \cup wu_0 \cup C'_{0,h-1} \cup u_{h-1}w' \cup Q_2 \cup z'v_\ell$, $C_{0,\ell} \cup v_0z \cup Q_1 \cup wu_0 \cup C'_{h-1,0} \cup u_{h-1}w' \cup Q_2 \cup z'v_\ell$, $C_{\ell,0} \cup v_0z \cup Q_1 \cup wu_0 \cup C'_{h-1,0} \cup u_{h-1}w' \cup Q_2 \cup z'v_\ell$ are 4 cycles of consecutive lengths in $G$.

Therefore, $H'$ is not 2-connected. Let $B_1, \dots, B_s$ be all end-blocks of $H'$ with cut-vertices $b_1, \dots, b_s$ respectively.

Assume that there exists $B_i$ such that $N_C(B_i - b_i) \neq \emptyset$. Without loss of generality, we may assume that $v_0$ has a neighbor $z$ in $B_i - b_i$. Let $z' \neq z$ be the neighbor of $v_\ell$ in $H'$. Since $H$ is 2-connected, we have that $N_{C'}(B_i - b_i) \neq \emptyset$. Without loss of generality, we may assume that $u_0$ has a neighbor $w$ in $B_i - b_i$. Similarly, whether $C'$ is of length 4 or not, $u_{h-1}$ contains a neighbor $w' \neq w$ in $H'$. Note that $z, w \in V(B_i - b_i)$. Using the block structure of $H'$, there exist two disjoint paths $R_1, R_2$ such that $R_1$ links $z$ and $w$ and $R_2$ links $z'$ and $w'$ in $H'$. Then $C_{0,\ell} \cup v_0z \cup R_1 \cup wu_0 \cup C'_{0,h-1} \cup u_{h-1}w' \cup R_2 \cup z'v_\ell$, $C_{\ell,0} \cup v_0z \cup R_1 \cup wu_0 \cup C'_{0,h-1} \cup u_{h-1}w' \cup R_2 \cup z'v_\ell$, $C_{0,\ell} \cup v_0z \cup R_1 \cup wu_0 \cup C'_{h-1,0} \cup u_{h-1}w' \cup R_2 \cup z'v_\ell$, $C_{\ell,0} \cup v_0z \cup R_1 \cup wu_0 \cup C'_{h-1,0} \cup u_{h-1}w' \cup R_2 \cup z'v_\ell$ are 4 cycles of consecutive lengths in $G$.

Therefore $N_C(\cup_{j\in[s]}(B_j - b_j)) = \emptyset$. Let $z_1$ be a neighbor of $v_0$ in $H'$. Since $G$ is $K_3$-free, at least one of $v_\ell, v_{\ell+1}$ has a neighbor other than $z_1$ in $H'$. Without loss of generality, we may assume that $v_\ell$ has a neighbor $z_2 \neq z_1$ in $H'$. Note that $z_1, z_2 \in H' - \cup_{j\in[s]}V(B_j - b_j)$. Using the block structure of $H'$, there are two end-blocks $B_1, B_2$ of $H'$ such that there exists disjoint paths $L_1, L_2$ from $\{z_1, z_2\}$ to $\{b_1, b_2\}$ in $H' - (V(B_1 - b_1) \cup V(B_2 - b_2))$. Without loss of generality, we may assume that $L_i$ links $b_i$ and $z_i$ for $i = 1, 2$.

Suppose that $C'$ is not cycle of length 4. Then every vertex of $\cup_{j\in[s]}V(B_j - b_j)$ has at most one neighbor in $V(C) \cup V(C')$. Note that $H$ is 2-connected. Therefore, there exists a vertex $w_j \in N_{V(B_j - b_j)}(C')$ for $j \in [s]$. It follows that $(B_j, b_j, w_j)$ is 2-connected and has minimum degree at least 3 for $j \in [s]$. Since $H$ is 2-connected, there exists a path $L$ from $w_1 \in V(B_1 - b_1)$ to $w_2 \in V(B_2 - b_2)$ whose internal vertices are in $C'$. Then by Theorem 2.2, there are two admissible paths $Q_{j,1}, Q_{j,2}$ between $b_j$ and $w_j$ in $B_j$ where $j = 1, 2$. Then at least 4 of $C_{0,\ell} \cup v_0z_1 \cup L_1 \cup Q_{1,\alpha} \cup L \cup Q_{2,\beta} \cup L_2 \cup z_2v_\ell$, $C_{\ell,0} \cup v_0z_1 \cup L_1 \cup Q_{1,\alpha} \cup L \cup Q_{2,\beta} \cup L_2 \cup z_2v_\ell$ for $\alpha, \beta \in [2]$ are cycles of consecutive lengths in $G$.

Therefore, $C'$ is a cycle of length 4. Suppose that $H'$ contains a vertex of degree one. Since it does not contain a neighbor on $C$ and $G$ is $K_3$-free, it has degree at most 3 in $G$, a contradiction. Therefore, we have that all end-blocks of $H'$ is 2-connected. Suppose that there exist $w_1 \in V(B_1 - b_1)$ which is adjacent to $u_t$ and $w_2 \in V(B_2 - b_2)$ which is adjacent to $u_{t+1}$ for some $t \in [4]$. Let $Q_i$ be a fixed path between $b_i$ and $w_i$ in $B_i$ for $i = 1, 2$. Then $C_{0,\ell} \cup v_0z_1 \cup L_1 \cup Q_1 \cup w_1u_tu_{t+1}w_2 \cup Q_2 \cup L_2 \cup z_2v_\ell$, $C_{0,\ell} \cup v_0z_1 \cup L_1 \cup Q_1 \cup w_1u_tu_{t-1}u_{t-2}u_{t+1}w_2 \cup Q_2 \cup L_2 \cup z_2v_\ell$, $C_{\ell,0} \cup v_0z_1 \cup L_1 \cup Q_1 \cup w_1u_tu_{t+1}w_2 \cup Q_2 \cup L_2 \cup z_2v_\ell$, $C_{\ell,0} \cup v_0z_1 \cup L_1 \cup Q_1 \cup w_1u_tu_{t-1}u_{t-2}u_{t+1}w_2 \cup Q_2 \cup L_2 \cup z_2v_\ell$ are 4 cycles of consecutive lengths in $G$. Therefore $N_{C'}((B_1 - b_1) \cup (B_2 - b_2)) \subseteq \{u_t, u_{t+2}\}$ for some $t \in \mathbb{Z}_4$. Hence $u_{t+1}$ has a neighbor $w' \in H' - (B_1 - b_1) \cup (B_2 - b_2)$. Using the block structure of $H'$, there exists $B_i$, where $i \in [2]$, such that there are two disjoint paths $N_1, N_2$ from $\{b_i, w'\}$ to $\{z_1, z_2\}$ in $H' - (B_1 - b_1) \cup (B_2 - b_2)$. Without loss of generality, we may assume that $i = 1$, $N_1$ links $z_1$ and $b_1$ and $N_2$ links $z_2$ and $w'$. Since $N_{C'}(B_1 - b_1) \subseteq \{u_t, u_{t+2}\}$, we may assume that $u_t \in N_{C'}(B_1 - b_1)$. Let $M$ be a fixed path from $b_1$ to $u_t$ in $G[B_1 \cup \{u_t\}]$. Then $C_{0,\ell} \cup v_0z_1 \cup N_1 \cup M \cup u_tu_{t+1}w' \cup N_2 \cup z_2v_\ell$, $C_{\ell,0} \cup v_0z_1 \cup N_1 \cup M \cup u_tu_{t+1}w' \cup N_2 \cup z_2v_\ell$, $C_{0,\ell} \cup v_0z_1 \cup N_1 \cup M \cup u_tu_{t-1}u_{t-2}u_{t+1}w' \cup N_2 \cup z_2v_\ell$, $C_{\ell,0} \cup v_0z_1 \cup N_1 \cup M \cup u_tu_{t-1}u_{t-2}u_{t+1}w' \cup N_2 \cup z_2v_\ell$ are 4 cycles of consecutive lengths in $G$. This completes the proof of Claim 1. ∎

Therefore $C' := u_0u_1 \dots u_{2h}u_0$ is an odd cycle, where the indices are taken under the additive group $\mathbb{Z}_{2h+1}$. By Lemma 4.6, we know that $N_G(C) \cap V(H') \neq \emptyset$.

Let $E_{C,C'} := \{e | e \text{ is an edge between } C \text{ and } C'\}$. Let $|E_{C,C'}| = m$ and $E_{C,C'} = \{e_1, e_2, \dots, e_m\}$. For any $e_p \in E_{C,C'}$, let $\{v_{\lambda_p}\} = V(e_p) \cap V(C)$ and $\{u_{\mu_p}\} = V(e_p) \cap V(C')$. By Lemma 4.4 and every vertex in $C'$ has at most one neighbor on $C$, we know that if $p \neq q$, then $\lambda_p \neq \lambda_q$ and $\mu_p \neq \mu_q$, that is edges between $C$ and $C'$ form a matching.

The remaining proof will be divided into two cases.

## 5.1 There exist some non-cut-vertices of $H'$ which have at least two neighbors in $V(C) \cup V(C')$ or $E_{C,C'} \neq \emptyset$.

Suppose that there exists a non-cut-vertex $x_1$ of $H_1 := H'$ which has at least two neighbors in $V(C) \cup V(C')$. Let $H_2 := H_1 - x_1$ and $X_1 = \{x_1\}$. If $H_i$ contains a non-cut-vertex $x_i$ which has at least two neighbors in $V(C) \cup V(C')$. Then we let $H_{i+1} := H_i - x_i$ and $X_i = X_{i-1} \cup \{x_i\}$. Note that every vertex of $H$ has at most one neighbor on $C$.

**Claim 2.** *For every $i$,*

1. *There exists a vertex $v_{\alpha_i}$ such that $v_{\alpha_i}$ is the unique neighbor of $x_i$ on $C$, and there exists a vertex $u_{\beta_i}$ such that $u_{\beta_i}$ is the unique neighbor of $x_i$ on $C'$.*
2. *$v_{\alpha_i} \neq v_{\lambda_p}$ and $u_{\beta_i} \neq u_{\mu_p}$ for every $p \in [m]$.*
3. *$v_{\alpha_j} \neq v_{\alpha_i}$ and $u_{\beta_j} \neq u_{\beta_i}$ for every $j < i$.*
4. *$X_i$ is an independent set of $G$. Moreover, every cut-vertex of $H'$ is also a cut-vertex of $H_{i+1}$.*

*Proof.* We proof by induction on $i$. Since $x_1$ is a non-cut-vertex of $H_1$, we know that $x_1$ has at most one neighbor on $C'$. Since every vertex of $H$ has at most one neighbor on $C$, we have that $x_1$ has at most one neighbor on $C$. Then $x_1$ has exactly one neighbor on $C$, denoted by $v_{\alpha_1}$, and exactly one neighbor on $C'$, denoted by $u_{\beta_1}$. Suppose that there exists $e_p \in E_{C,C'}$ such that $v_{\alpha_1} = v_{\lambda_p}$ or $u_{\beta_1} = u_{\mu_p}$. Since $G$ is $K_3$-free, we may assume that $v_{\alpha_1} = v_{\lambda_p}$ and $u_{\beta_1} \neq u_{\mu_p}$. Note that $x_1$ has exactly one neighbor on $C$ and edges between $C$ and $C'$ are a matching. Since vertex on $C$ has degree at least 4, $v_{\alpha_1+\ell}$ has a neighbor $z$ in $H_2$. Let $Q'_o$ be the odd path between $u_{\mu_p}$ and $u_{\beta_1}$ in $C'$ and $2s + 1$ denote the

length of $Q'_o$. We may assume that $\beta_1 = \mu_p + 2s + 1$. Since $u_{\beta_1} \neq u_{\mu_p+s}$ is the unique neighbor fo $x_1$ on $C'$, there exists a vertex $w$ be a neighbor of $u_{\mu_p+s}$ in $H_2$. Clearly, there exists a fixed path $L_1$ between $z$ and $w$ disjoint from $V(C) \cup \{x_1\} \cup V(C')$. Then $C_{\alpha_1,\alpha_1+\ell} \cup v_{\alpha_1+\ell}z \cup L_1 \cup u_{\mu_p+s}w \cup C'_{\mu_p,\mu_p+s} \cup u_{\mu_p}v_{\alpha_1}$, $C_{\alpha_1+\ell,\alpha_1} \cup v_{\alpha_1+\ell}z \cup L_1 \cup u_{\mu_p+s}w \cup C'_{\mu_p,\mu_p+s} \cup u_{\mu_p}v_{\alpha_1}$, $C_{\alpha_1,\alpha_1+\ell} \cup v_{\alpha_1+\ell}z \cup L_1 \cup u_{\mu_p+s}w \cup C'_{\mu_p+s,\beta_1} \cup u_{\beta_1}x_1v_{\alpha_1}$, $C_{\alpha_1+\ell,\alpha_1} \cup v_{\alpha_1+\ell}z \cup L_1 \cup u_{\mu_p+s}w \cup C'_{\mu_p+s,\beta_1} \cup u_{\beta_1}x_1v_{\alpha_1}$ are 4 cycles of consecutive lengths in $G$. Therefore, $v_{\alpha_1} \neq v_{\lambda_p}$ and $u_{\beta_1} = u_{\mu_p}$. Similarly, we could find 4 cycles of consecutive lengths in $G$. Hence claim 2 is true for $i = 1$. Clearly, $X_1$ is an independent set of $G$, which implies that every cut-vertex of $H_1$ is also a cut-vertex of $H_2$. We assume that $i \geq 2$ and for every $j < i$ the claim is true.

Since every cut-vertex of $H'$ is also a cut-vertex of $H_i$, we have that $x_i$ is not a cut vertex in $H'$. Since every vertex of $H$ has at most one neighbor on $C$, there exists a vertex $v_{\alpha_i}$ such that $v_{\alpha_i}$ is the unique neighbor of $x_i$ on $C$, and there exists a vertex $u_{\beta_i}$ such that $u_{\beta_i}$ is the unique neighbor of $x_i$ on $C'$.

Suppose that there exists $e_p \in E_{C,C'}$ such that $v_{\alpha_i} = v_{\lambda_p}$ or $u_{\beta_i} = u_{\mu_p}$. Since $G$ is $K_3$-free, we may assume that $v_{\alpha_i} = v_{\lambda_p}$ and $u_{\beta_i} \neq u_{\mu_p}$. Note that $x_i$ has exactly one neighbor on $C$ and edges between $C$ and $C'$ are a matching. By induction hypothesis, $v_{\alpha_i+\ell}$ has a neighbor $z_2$ in $H_{i+1}$. Let $Q'_o$ be the odd path between $u_{\mu_p}$ and $u_{\beta_i}$ in $C'$ and $2s+1$ denote the length of $Q'_o$. We may assume that $\beta_i = \mu_p + 2s + 1$. Note that $u_{\mu_p+s}$ is not adjacent to $x_i$. By Claim 4.4 and induction hypothesis, $u_{\mu_p+s}$ has a neighbor $w_2$ in $H_{i+1}$. Clearly, there exists a fixed path $L_2$ between $z_2$ and $w_2$ disjoint from $V(C) \cup \{x_i\} \cup V(C')$. Then $C_{\alpha_i,\alpha_i+\ell} \cup v_{\alpha_i+\ell}z_2 \cup L_2 \cup u_{\mu_p+s}w_2 \cup C'_{\mu_p,\mu_p+s} \cup u_{\mu_p}v_{\alpha_i}$, $C_{\alpha_i+\ell,\alpha_i} \cup v_{\alpha_i+\ell}z_2 \cup L_2 \cup u_{\mu_p+s}w_2 \cup C'_{\mu_p,\mu_p+s} \cup u_{\mu_p}v_{\alpha_i}$, $C_{\alpha_i,\alpha_i+\ell} \cup v_{\alpha_i+\ell}z_2 \cup L_2 \cup u_{\mu_p+s}w_2 \cup C'_{\mu_p+s,\beta_i} \cup u_{\beta_i}x_iv_{\alpha_i}$, $C_{\alpha_i+\ell,\alpha_i} \cup v_{\alpha_i+\ell}z_2 \cup L_2 \cup u_{\mu_p+s}w_2 \cup C'_{\mu_p+s,\beta_i} \cup u_{\beta_i}x_iv_{\alpha_i}$ are 4 cycles of consecutive lengths in $G$. Therefore, $v_{\alpha_i} \neq v_{\lambda_p}$ and $u_{\beta_i} = u_{\mu_p}$. Similarly, we could find 4 cycles of consecutive lengths in $G$. Therefore for any $e_j \in E_{C,C'}$ we have that $v_{\alpha_i} \neq v_{\lambda_j}$ and $u_{\beta_i} \neq u_{\mu_j}$.

Suppose that there exists $x_j$ for $j < i$ such that $v_{\alpha_i} = v_{\alpha_j}$. Assume that $u_{\beta_i} = u_{\beta_j}$. Since vertex on $C$ has degree at least 4 and edges between $C, C'$ are a matching, by induction hypothesis, $v_{\alpha_i+\ell}$ has a neighbor $z_3$ in $H_{i+1}$. Since $x_i$ is a non-cut-vertex of $H_i$, $x_i$ has a neighbor $w_3$ in $H_{i+1}$. Let $L_3$ be a fixed path between $z_3$ and $w_3$ in $H_{i+1}$. Then $C_{\alpha_i,\alpha_i+\ell} \cup v_{\alpha_i+\ell}z_3 \cup L_3 \cup w_3x_iv_{\alpha_i}$, $C_{\alpha_i+\ell,\alpha_i} \cup v_{\alpha_i+\ell}z_3 \cup L_3 \cup w_3x_iv_{\alpha_i}$, $C_{\alpha_i,\alpha_i+\ell} \cup v_{\alpha_i+\ell}z_3 \cup L_3 \cup w_3x_iu_{\beta_i}x_jv_{\alpha_i}$, $C_{\alpha_i+\ell,\alpha_i} \cup v_{\alpha_i+\ell}z_3 \cup L_3 \cup w_3x_iu_{\beta_i}x_jv_{\alpha_i}$ are 4 cycles of consecutive lengths in $G$. Therefore $u_{\beta_i} \neq u_{\beta_j}$. Since vertex on $C$ has degree at least 4 and edges between $C, C'$ are a matching, by induction hypothesis, $v_{\alpha_i+\ell}$ has a neighbor $z_4$ in $H_{i+1}$. Let $Q'_e$ be the even path between $u_{\beta_i}$ and $u_{\beta_j}$ in $C'$ and $2s$ denote the length of $Q'_e$. We may assume that $\beta_j = \beta_i + 2s$. Since every vertex of $C'$ has degree at least 4, $u_{\beta_i+s-1}$ has a neighbor $w_4$ in $H' - \{x_i, x_j\}$. By induction hypothesis every vertex of $X_i - \{x_i, x_j\}$ has a neighbor in $H_{i+1}$. So there exists a fixed path $L_4$ between $z_4$ and $w_4$ disjoint from $V(C) \cup \{x_i, x_j\} \cup V(C')$. Then $C_{\alpha_i,\alpha_i+\ell} \cup v_{\alpha_i+\ell}z_4 \cup L_4 \cup u_{\beta_i+s-1}w_4 \cup C'_{\beta_i,\beta_i+s-1} \cup u_{\beta_i}x_iv_{\alpha_i}$, $C_{\alpha_i+\ell,\alpha_i} \cup v_{\alpha_i+\ell}z_4 \cup L_4 \cup u_{\beta_i+s-1}w_4 \cup C'_{\beta_i,\beta_i+s-1} \cup u_{\beta_i}x_iv_{\alpha_i}$, $C_{\alpha_i,\alpha_i+\ell} \cup v_{\alpha_i+\ell}z_4 \cup L_4 \cup u_{\beta_i+s-1}w_4 \cup C'_{\beta_i+s-1,\beta_j} \cup u_{\beta_j}x_jv_{\alpha_i}$, $C_{\alpha_i+\ell,\alpha_i} \cup v_{\alpha_i+\ell}z_4 \cup L_4 \cup u_{\beta_i+s-1}w_4 \cup C'_{\beta_i+s-1,\beta_j} \cup u_{\beta_j}x_jv_{\alpha_i}$ are 4 cycles of consecutive lengths in $G$. Therefore $v_{\alpha_i} = v_{\alpha_j}$. If $u_{\beta_i} \neq u_{\beta_j}$, then we could similarly find 4 cycles of consecutive lengths in $G$. So $v_{\alpha_j} \neq v_{\alpha_i}$ and $u_{\beta_j} \neq u_{\beta_i}$ for every $j < i$.

Suppose that $x_i$ has a neighbor $x_q$ in $X_{i-1}$. Since $G$ is $K_3$-free, we have that $v_{\alpha_i} \neq v_{\alpha_q}$ and $u_{\beta_i} \neq u_{\beta_q}$. Let $Q_e$ be the even path between $v_{\alpha_i}$ and $v_{\alpha_q}$ in $C$ and $2r$ denote the length of $Q_e$. We may assume that $\alpha_q = \alpha_i + 2r$. Since vertex on $C$ has degree at least 4 and edges between $C, C'$ are a matching, by induction hypothesis, $v_{\alpha_i+r}$ has a neighbor $z_5$ in $H_{i+1}$. Let $Q'_e$ be the even path between $u_{\beta_i}$ and $u_{\beta_q}$ in $C'$ and $2s$ denote the length of $Q'_e$. We may assume that $\beta_q = \beta_i + 2s$. Since $u_{\beta_i}$ is the unique neighbor of $x_i$ on $C'$ and vertex of $C'$ has degree at least 4, by induction hypothesis, $u_{\beta_i+s-1}$ has a neighbor $w_5$ in $H_{i+1}$. By induction hypothesis every vertex of $X_i - \{x_i, x_q\}$ has a neighbor in $H_{i+1}$. So there exists a fixed path $L_5$ between $z_5$ and $w_5$ disjoint from $V(C) \cup \{x_i, x_q\} \cup V(C')$. Then $C_{\alpha_i,\alpha_i+r} \cup v_{\alpha_i+r}z_5 \cup L_5 \cup u_{\beta_i+s-1}w_5 \cup C'_{\beta_i,\beta_i+s-1} \cup u_{\beta_i}x_iv_{\alpha_i}$, $C_{\alpha_i+r,\alpha_q} \cup v_{\alpha_i+r}z_5 \cup L_5 \cup u_{\beta_i+s-1}w_5 \cup$

$C'_{\beta_i,\beta_i+s-1} \cup u_{\beta_i}x_ix_qv_{\alpha_q}$, $C_{\alpha_i+r,\alpha_q} \cup v_{\alpha_i+r}z_5 \cup L_5 \cup u_{\beta_i+s-1}w_5 \cup C'_{\beta_i+s-1,\beta_q} \cup u_{\beta_q}x_qv_{\alpha_q}$, $C_{\alpha_i,\alpha_i+r} \cup v_{\alpha_i+r}z_5 \cup L_5 \cup u_{\beta_i+s-1}w_5 \cup C'_{\beta_i+s-1,\beta_q} \cup u_{\beta_q}x_qx_iv_{\alpha_i}$ are 4 cycles of consecutive lengths in $G$. Therefore $X_i$ is an independent set of $G$. Since $H_{i+1} = H' \setminus X_i$ is connected and the minimal degree of $H'$ is at least two, we know that every cut-vertex of $H'$ is also a cut-vertex of $H_{i+1}$. This completes the proof of Claim 2. ∎

We do this until the remaining graph satisfying that every non-cut-vertex of it contains at most one neighbor in $V(C) \cup V(C')$. Let $t$ denote the number of vertices that we delete. Let $X = X_t$ and $H'' = H_{t+1}$.

**Claim 3.** *Every non-cut-vertex of $H''$ has at most one neighbor in $V(C) \cup X \cup V(C')$.*

*Proof.* Suppose there exists a non-cut-vertex $v$ of $H''$ such that $v$ has at least two neighbor in $V(C) \cup X \cup V(C')$. By Claim 2, we have that every non-cut-vertex of $H''$ is the non-cut-vertex of $H'$. It follows that every non-cut-vertex of $H''$ has at most one neighbor in $V(C) \cup V(C')$. Suppose that $v$ has a neighbor $x_i$ in $X$ and a neighbor $u_\gamma$ on $C'$. Since $G$ is $K_3$-free, we have that $u_\gamma \neq u_{\beta_i}$. Let $Q'_o$ be the even path between $u_\gamma$ and $u_{\beta_i}$ in $C'$ and $2s+1$ denote the length of $Q'_o$. We may assume that $\gamma = \beta_i + 2s + 1$. By Claim 2 and $G$ is $K_3$-free, $u_{\beta_i+s}$ has a neighbor $w$ in $H' - \{v\}$. Since vertex on $C$ has degree at least 4, by Claim 2, $v_{\alpha_i+\ell}$ has a neighbor $z$ in $H' - \{v\}$. Note that every vertex of $X$ has at least two neighbors in $H''$ and $v$ is a non-cut-vertex of $H''$. There exists a fixed path $L$ between $z$ and $w$ disjoint from $V(C) \cup \{x_i, v\} \cup V(C')$. Then $C_{\alpha_i,\alpha_i+\ell} \cup v_{\alpha_i+\ell}z \cup L \cup u_{\beta_i+s}w \cup C'_{\beta_i,\beta_i+s} \cup u_{\beta_i}x_iv_{\alpha_i}$, $C_{\alpha_i+\ell,\alpha_i} \cup v_{\alpha_i+\ell}z \cup L \cup u_{\beta_i+s}w \cup C'_{\beta_i,\beta_i+s} \cup u_{\beta_i}x_iv_{\alpha_i}$, $C_{\alpha_i,\alpha_i+\ell} \cup v_{\alpha_i+\ell}z \cup L \cup u_{\beta_i+s}w \cup C'_{\beta_i+s,\gamma} \cup u_\gamma vx_iv_{\alpha_i}$, $C_{\alpha_i+\ell,\alpha_i} \cup v_{\alpha_i+\ell}z \cup L \cup u_{\beta_i+s}w \cup C'_{\beta_i+s,\gamma} \cup u_\gamma vx_iv_{\alpha_i}$ are 4 cycles of consecutive lengths in $G$.

Suppose that $v$ has a neighbor in $X$ and a neighbor on $C$. Then we could similarly find 4 cycles of consecutive lengths in $G$.

Therefore $N_G(v) \cap (V(C) \cup X \cup V(C')) \subseteq X$. Let $x_p, x_q$ be two neighbors of $v$ in $X$. Let $Q_o$ be the odd path between $v_{\alpha_p}$ and $v_{\alpha_q}$ in $C$ and $2r+1$ denote the length of $Q_o$. We may assume that $\alpha_q = \alpha_p + 2r + 1$. By Claim 2, $v_{\alpha_p+r}$ has a neighbor $z'$ in $H'' - \{v\}$. Let $Q'_e$ be the even path between $u_{\beta_p}$ and $u_{\beta_q}$ in $C'$ and $2s$ denote the length of $Q_o$. We may assume that $\beta_q = \beta_p + 2s$. By Claim 2, $u_{\beta_p+s}$ has a neighbor $w'$ in $H'' - \{v\}$. Since $v$ is a non-cut-vertex of $H''$, there exists a fixed path $L'$ between $z'$ and $w'$ in $H'' - \{v\}$. Then $C_{\alpha_p,\alpha_p+r} \cup v_{\alpha_p+r}z' \cup L' \cup u_{\beta_p+s}w' \cup C'_{\beta_p,\beta_p+s} \cup u_{\beta_p}x_pv_{\alpha_p}$, $C_{\alpha_p+r,\alpha_q} \cup v_{\alpha_p+r}z' \cup L' \cup u_{\beta_p+s}w' \cup C'_{\beta_p+s,\beta_q} \cup u_{\beta_q}x_qv_{\alpha_q}$, $C_{\alpha_p,\alpha_p+r} \cup v_{\alpha_p+r}z' \cup L' \cup u_{\beta_p+s}w' \cup C'_{\beta_p+s,\beta_q} \cup u_{\beta_q}x_qvx_pv_{\alpha_p}$, $C_{\alpha_p+r,\alpha_q} \cup v_{\alpha_p+r}z' \cup L' \cup u_{\beta_p+s}w' \cup C'_{\beta_p,\beta_p+s} \cup u_{\beta_p}x_pvx_qv_{\alpha_q}$ are 4 cycles of consecutive lengths in $G$. This completes the proof of Claim 3. ∎

Let $E'_{C,C'} := \{v_{\alpha_i}x_iv_{\beta_i}, i \in [t]\}$. Since $G$ has minimum degree at least 4, by Claim 3, we have that every non-cut-vertex of $H''$ has degree at least 3.

**Claim 4.** $E_{C,C'} \cup E'_{C,C'} = \emptyset$.

*Proof.* Let $P \in E_{C,C'} \cup E'_{C,C'}$ be a path linking $C$ and $C'$. Let $V(P) \cap V(C) = \{v_p\}$ and $V(P) \cap V(C') = \{u_p\}$. Suppose that $H''$ is 2-connected. Since $G$ has minimum degree at least 4, by Claim 2, $v_{p+\ell}$ has a neighbor $z \in V(H'')$ and $u_{p+h}$ has a neighbor $w \in V(H'')$. By the definition of $X$, we have that $z \neq w$. Clearly, $(H'', z, w)$ is 2-connected of minimum degree at least 3. By Theorem 2.2, there exist two admissible paths $Q_1, Q_2$ between $z$ and $w$ in $H''$. Then at least 4 of $C_{p,p+\ell} \cup v_{p+\ell}z \cup Q_i \cup u_{p+h}w \cup C'_{p,p+h} \cup P$, $C_{p,p+\ell} \cup v_{p+\ell}z \cup Q_i \cup u_{p+h}w \cup C'_{p+h,p} \cup P$, $C_{p+\ell,p} \cup v_{p+\ell}z \cup Q_i \cup u_{p+h}w \cup C'_{p,p+h} \cup P$, $C_{p+\ell,p} \cup v_{p+\ell}z \cup Q_i \cup u_{p+h}w \cup C'_{p+h,p} \cup P$, for $i = 1, 2$ are cycles of consecutive lengths in $G$.

Therefore $H''$ is not 2-connected. Let $B_1, \ldots, B_s$ be all end-blocks of $H''$ with cut-vertices $b_1, \ldots, b_s$ respectively. Note that $B_i$ is 2-connected for $i \in [s]$. Since $H$ is 2-connected, by Lemma 4.5 and Claim

3, there exists (i) $x_j$ such that $N_{C\cup X}(\cup_{i\in[s]}(B_i - b_i)) \subseteq \{x_j, u_{\beta_j}\}$, or (ii) $u_d$ such that $N_{C\cup X}(\cup_{i\in[s]}(B_i - b_i)) = \{u_d\}$. For the former case, let $w_i \in N_{B_i - b_i}(\{x_j, u_{\beta_j}\})$ and for the latter case let $w_i \in N_{B_i-b_i}(u_d)$. Since $(B_i, b_i, w_i)$ is 2-connected of minimum degree at least 3, by Theorem 2.2, there exist two admissible paths $Q_{i,1}, Q_{i,2}$ with difference one from $b_i$ to $w_i$ in $B_i$.

By Claim 2, there exists a path $Q$ of length at most 2 from $v_{p+\ell}$ to $H''$, which internal vertices are in $X - \{x_j\}$. Suppose that another end $a$ of $Q$ is in $\cup_{j\in[s]}(V(B_j - b_j))$. Without loss of generality, we may assume that $a$ is in $B_1 - b_1$. It is clear that $(B_1, a, b_1)$ is 2-connected of minimum degree at least 3. By Theorem 2.2, there are 2 admissible paths $R_1, R_2$ between $a$ and $b_1$ in $B_1$. Let $L_1$ be a fixed path between $b_1$ and $b_2$ in $H'' - (B_1 - b_1) \cup (B_2 - b_2)$. Note that there exists a fixed path $N_1$ between $w_2$ and $v_p$ internally disjoint from $C \cup H'' \cup Q$. Then at least 4 of $C_{p,p+\ell} \cup Q \cup R_\alpha \cup L_1 \cup Q_{2,\beta} \cup N_1$, $C_{p+\ell,p} \cup Q \cup R_\alpha \cup L_1 \cup Q_{2,\beta} \cup N_1$, where $\alpha, \beta = 1, 2$ are consecutive cycles in $G$. Therefore $a$ is in $V(H'') - (\cup_{j\in[s]}(B_j - b_j))$.

Similarly, there exists a path $R$ of length at most 2 from $v_{p+\ell+1}$ to $H''$, which internal vertices are in $X - \{x_j\}$. Let $a''$ be another end of $R$. By symmetry, we have that $a'' \in V(H'') - (\cup_{j\in[s]}(B_j - b_j))$. By Claim 2 and $G$ has minimum degree at least 4, we may assume that $a' \neq a''$. Using the block structure of $H''$, there exist $B_i$ and $B_j$ such that there exist two disjoint paths $T_1$ from $b_i$ to $a'$ and $T_2$ from $b_j$ to $a''$ in $H'' - (\cup_{j\in[s]}(B_j - b_j))$. Note that there is a fixed path $N_2$ between $w_i$ and $w_j$ internally disjoint from $C \cup H''$. Then $Q_{i,\alpha} \cup T_1 \cup a'v_{p+\ell} \cup C_{p+\ell,p+\ell+1} \cup a''v_{p+\ell+1} \cup T_2 \cup Q_{j,\beta} \cup N_2$ are 3 cycles of consecutive lengths in $G$ and $Q_{i,\alpha} \cup T_1 \cup a'v_{p+\ell} \cup C_{p+\ell+1,p+\ell} \cup a''v_{p+\ell+1} \cup T_2 \cup Q_{j,\beta} \cup N_2$ are 3 cycles of consecutive lengths in $G$, where $\alpha, \beta = 1, 2$. Since $|C_{p+\ell,p+\ell+1}|$ and $|C_{p+\ell+1,p+\ell}|$ are of different parity, one of above two classes are desired cycles of consecutive lengths. This completes the proof of Claim 4. ∎

### 5.2 Every non-cut-vertex of $H'$ has at most one neighbor in $V(C) \cup V(C')$ and there is no edge between $C$ and $C'$.

Suppose that $H'$ is not 2-connected. Let $B_1, \dots, B_s$ be all end-blocks of $H''$ with cut-vertices $b_1, \dots, b_s$ respectively. Note that $B_i$ is 2-connected of minimum degree at least 3 for $i \in [s]$ and $C'$ is odd. By Lemma 4.5, there exists an vertex $u_d$ on $C'$ such that for every $i \in [s]$, $N_{C'}(B_i - b_i) = \{u_d\}$ and there are 2 admissible paths $Q_{i,1}, Q_{i,2}$ between $u_d$ and $b_i$ in $B_i$ satisfying that $|E(Q_{i,1})| - |E(Q_{i,2})| = 1$.

Suppose that there exist $v_i$ and $v_{i+\ell}$ on $C$ such that $v_i$ has a neighbor $y_1$ in $B_1 - b_1$ and $v_{i+\ell}$ has a neighbor $y_2$ in $B_2 - b_2$. Clearly, $(B_j, y_j, b_j)$ is 2-connected of minimum degree at least 3. By Theorem 2.2, there are 2 admissible paths $Q'_{j,1}, Q'_{j,2}$ between $y_j$ and $b_j$ in $B_j$ for $j = 1, 2$. Let $L_1$ be a fixed path between $b_1$ and $b_2$ in $H'' - ((B_1 - b_1) \cup (B_2 - b_2))$. Then at least 4 of $C_{i,i+\ell} \cup v_i y_1 \cup Q'_{1,\alpha} \cup L_1 \cup Q'_{2,\beta} \cup v_{i+\ell} y_2$, $C_{i+\ell,i} \cup v_i y_1 \cup Q'_{1,\alpha} \cup L_1 \cup Q'_{2,\beta} \cup v_{i+\ell} y_2$ where $\alpha, \beta = 1, 2$, are cycles of consecutive lengths in $G$. Therefore, there is no such pair of vertices in $C$.

Let $z$ be the neighbor of $u_{d+h}$ in $H'$. Note that $z \in V(H') - \cup_{i\in[s]}(V(B_i - b_i))$. Assume that $z$ is in the block $B$ of $H'$. Let $b$ be a cut-vertex other than $z$ of $B$ in $H'$. Let $F$ be the component of $H' - b$ containing $z$. Suppose that there exist $v_i$ and $v_{i+\ell}$ such that $v_i$ has a neighbor $y_1$ in $F_1$ and $v_{i+\ell}$ has a neighbor $y_2$ in $H' - F$. Note that at least one of $y_1, y_2$ are not in $\cup_{j\in[s]}(V(B_j - b_j))$. Without loss of generality, we may assume that $y_1$ is not in $\cup_{j\in[s]}(V(B_j - b_j))$. Without loss of generality, we may assume that $(B_1 - b_1) \subseteq F$. Using the block structure of $H'$, there exist three internally disjoint paths $T_1, T_2$ in $H'$ such that $T_1$ links $y_1$ and $b_1$, $T_2$ links $y_2$ and $z$. Then at least 4 of $C_{i,i+\ell} \cup v_i y_1 \cup T_1 \cup Q_{1,\alpha} \cup C'_{d,d+h} \cup u_{d+h} z \cup T_2 \cup y_2 v_{i+\ell}$, $C_{i+\ell,i} \cup v_i y_1 \cup T_1 \cup Q_{1,\alpha} \cup C'_{d,d+h} \cup u_{d+h} z \cup T_2 \cup y_2 v_{i+\ell}$, $C_{i,i+\ell} \cup v_i y_1 \cup T_1 \cup Q_{1,\alpha} \cup C'_{d+h,d} \cup u_{d+h} z \cup T_2 \cup y_2 v_{i+\ell}$, $C_{i+\ell,i} \cup v_i y_1 \cup T_1 \cup Q_{1,\alpha} \cup C'_{d+h,d} \cup u_{d+h} z \cup T_2 \cup y_2 v_{i+\ell}$ where $\alpha = 1, 2$, are cycles of consecutive lengths in $G$.

Therefore there exists a component $F'$ of $H' - b$ such that $N_G(C) \cap F' = \emptyset$. Without loss of generality, we may assume that $(B_1 - b_1) \subseteq F'$. It follows that $(B_1, b_1, u_d)$ is 2-connected of minimum degree at least 4. By Theorem 2.2, there are 3 admissible paths $Q''_1, Q''_2, Q''_3$ between $u_d$ and $b_1$ in $B_1$.

Let $L_2$ be a fixed path between $b_1$ and $z$ in $H' - (B_1 - b_1)$. Then at least 4 of $C'_{d,d+h} \cup u_{d+h}z \cup L_2 \cup Q''_\alpha$, $C'_{d+h,d} \cup u_{d+h}z \cup L_2 \cup Q''_\alpha$ where $\alpha = 1, 2, 3$, are cycles of consecutive lengths in $G$.

Hence, $H'$ is 2-connected and has minimum degree at least 3. This completes the proof of Lemma 5.1. ∎

# 6 Proof of Theorem 1.2

Now, we are in a position to prove Theorem 1.2. We need the following well-known theorem proved by Thomassen and Toft.

**Theorem 6.1** (Thomassen and Toft [5]). *Every 2-connected graph $G$ of minimum degree at least three contains a non-separating induced cycle.*

We need the following lemma on non-separating odd cycles from [4].

**Lemma 6.2** ( [4] Lemma 5.1). *Let $G$ be a graph of minimum degree at least four. If $G$ contains a non-separating induced odd cycle, then $G$ contains a non-separating induced odd cycle $C$, denoted by $v_0v_1...v_{2s}v_0$, such that either*

1. *$C$ is a triangle, or*
2. *for every non-cut-vertex $v$ of $G - V(C)$, $|N_G(v) \cap V(C)| \leq 2$, and the equality holds if and only if $N_G(v) \cap V(C) = \{v_i, v_{i+2}\}$ for some $i$, where the indices are taken under the additive group $\mathbb{Z}_{2s+1}$.*

*Proof of Theorem 1.2.* It suffices to consider 5-critical graphs $G$. By Theorems 2.3 and 2.1, we have that $G$ is $K_3$-free and contains a non-separating induced odd cycle. Let $C_1 := v_0v_1 \dots v_{2l}v_0$ be the minimum non-separating induced odd cycle of $G$, where $\ell \geq 2$ and the indices are taken under the additive group $\mathbb{Z}_{2\ell+1}$ and let $H_1 = G - V(C_1)$. By Lemma 6.2 and Lemma 4.2, we have that every non-cut-vertex of $H_1$ has at most one neighbor on $C$.

Suppose that $H_1$ is not 2-connected. Let $B_1, \dots, B_s$ be all end-blocks of $H_1$ with cut-vertices $b_1, \dots, b_s$ respectively. Note that $B_i$ is 2-connected for $i \in [s]$. By Lemma 4.5, there exists an vertex $v_d$ on $C'$ such that for every $i \in [s]$, $N_{C'}(B_i - b_i)$ and there are 2 admissible paths $Q_{i,1}, Q_{i,2}$ between $v_d$ and $b_i$ in $G[B_i \cup \{v_d\}]$ satisfying that $|E(Q_{i,1})| - |E(Q_{i,2})| = 1$. It follows that $(G[B_1 \cup \{v_d\}], v_d, b_1)$ is 2-connected of minimum degree at least 4. By Theorem 2.2, there exist 3 admissible paths $R_1, R_2, R_3$ between $v_d$ and $b_1$ in $G[B_1 \cup \{v_d\}]$. Let $w$ be the neighbor of $v_{d+\ell}$ in $H_1$. Note that $w \notin (B_1 - b_1)$. Let $L$ be a fixed path between $w$ and $b_1$ in $H_1 - (B_1 - b_1)$. Then at least 4 of $R_j \cup L \cup wv_{d+\ell} \cup C_{d,d+\ell}$, $R_j \cup L \cup wv_{d+\ell} \cup C_{d+\ell,d}$, where $j = 1, 2, 3$ are cycles of consecutive lengths in $G$.

Therefore $H_1$ is 2-connected of minimum degree at least 3. By Theorem 6.1, $H_1$ contains a non-separating induced cycle $C_2$. We choose $C_2$ such that $C_2$ is minimum. By Lemma 5.1, we know that $H_2 := H_1 - V(C_2)$ is 2-connected and has minimum degree at least 3, $C_2$ is odd and there is no edge between $C_1$ and $C_2$. Assume that we have found induced odd cycles $C_1, C_2, \dots, C_m$ and $H_m$ where $m \geq 2$, such that $H_m$ is 2-connected and every non-cut-vertex of $H_m$ has at most one neighbor in $\cup_{i \in [m]} C_i$ and there is no edge between $C_i$ and $C_j$ for $1 \leq i < j \leq m$. By Theorem 6.1, $H_m$ contains a non-separating induced cycle. Let $C_{m+1}$ be the minimum non-separating induced cycle of $H_m$ and $H_{m+1} := H_m - V(C_{m+1})$. Note that every vertex of $C_{m+1}$ has at least one neighbor in $H_{m+1}$ and every non-cut-vertex of $H_{m+1}$ has at most one neighbor on $C_{m+1}$ unless $C_{m+1}$ is a cycle of length 4.

By Lemma 4.4, we know that for every $i \in [m]$,

(i) if $C_{m+1}$ is even, then $N_G(C_i) \subseteq V(H_{m+1})$.

(ii) if $C_{m+1}$ is odd, then $N_G(C_i) \subseteq V(C_{m+1})$ or edges(if exist) between $C_i$ and $C_{m+1}$ in $G$ are a matching.

Let $G_i := G - V(C_i)$. Note that $G_i$ is 2-connected.

**Claim 5.** *$C_{m+1}$ is a non-separating induced cycle of $G_i$ for every $i < m + 1$.*

*Proof.* By Lemma 4.4, we know that $C_{m+1}$ is odd. Let $C' = C_{m+1} := u_0u_1 \dots u_{2h}u_0$, where the indices are taken under the additive group $\mathbb{Z}_{2h+1}$. Suppose to the contrary that exists $x \in [m]$ such that $N_G(C_x) \cap V(H_{m+1}) = \emptyset$. Since there is no edge between $C_x$ and $\cup_{i\in([m]-x)}C_i$, we have that $N_G(C_x) \subseteq V(C_{m+1})$. Let $X := \{x \in [m] | N_G(C_x) \subseteq V(C'\}$. Let $G' := G - \cup_{j\in X}V(C_j)$. Then $C_{m+1}$ is a non-separating induced cycle of $G'$.

We will show that every non-cut-vertex of $G' - V(C')$ has at most one neighbor on $C_{m+1}$. By Lemma 4.4, every vertex of $\cup_{j\in[m]}C_j$ has at most one neighbor on $C'$. By the minimality of $C_{m+1}$, every non-cut-vertex of $H_{m+1}$ has at most one neighbor on $C'$. Suppose that a cut-vertex $b$ of $H_{m+1}$ is not a cut-vertex in $G' - V(C')$ and $b$ has two neighbors $u_\alpha, u_\beta$ on $C'$. Let $F_1, \dots, F_n$ be all components of $H_{m+1} - \{b\}$. Let $Q'_e$ be the even path between $u_\alpha$ and $u_\beta$ in $C'$ and $2s$ denote the length of $Q'_e$. We may assume that $\beta = \alpha + 2s$. By Lemma 4.2, we have that $s \geq 2$ and at least one of $u_{\alpha+s-1}, u_{\alpha+s+1}$ has a neighbor $w \neq b$ in $H_{m+1}$. Without loss of generality, we may assume that $u_{\alpha+s-1}$ and $w$ are adjacent in $G$ and $w \in V(F_1)$. It follows that there exist $j \in ([m] - X)$ such that $N_{F_1}(C_j) \neq \emptyset$ and $N_{H_{m+1}-F_1}(C_j) \neq \emptyset$. Let $C = C_j := v_0v_1 \dots v_{2l}v_0$, where the indices are taken under the additive group $\mathbb{Z}_{2\ell+1}$. Since $C_j$ is odd, by Lemma 4.1, we may assume that $v_0$ has a neighbor $z_1$ in $F_1$ and $v_\ell$ has a neighbor $z_2$ in $H_{m+1} - F_1$. Using the block structure, there exist two disjoint paths $L_1$ and $L_2$ such that $L_1$ links $z_1$ and $w$ in $H_{m+1}$ and $L_2$ links $z_2$ and $b$ in $H_{m+1}$. Then $C_{0,\ell} \cup v_0z_1 \cup L_1 \cup wu_{\alpha+s-1} \cup C'_{\alpha,\alpha+s-1} \cup u_\alpha b \cup L_2 \cup z_2v_\ell$, $C_{\ell,0} \cup v_0z_1 \cup L_1 \cup wu_{\alpha+s-1} \cup C'_{\alpha,\alpha+s-1} \cup u_\alpha b \cup L_2 \cup z_2v_\ell$, $C_{0,\ell} \cup v_0z_1 \cup L_1 \cup wu_{\alpha+s-1} \cup C'_{\alpha+s-1,\beta} \cup u_\beta b \cup L_2 \cup z_2v_\ell$, $C_{\ell,0} \cup v_0z_1 \cup L_1 \cup wu_{\alpha+s-1} \cup C'_{\alpha+s-1,\beta} \cup u_\beta b \cup L_2 \cup z_2v_\ell$ are 4 cycles of consecutive cycles. Therefore every non-cut-vertex of $G' - V(C')$ has at most one neighbor on $C'$.

Hence, for every $x \in X$, $C_x, C_{m+1}, G' - V(C_{m+1})$ satisfy the conditions of Lemma 4.6. It follows that $N_G(C_x) \cap V(H_{m+1}) \neq \emptyset$ for every $x \in X$. This completes the proof of Claim 5. ∎

Since $C_{m+1}$ is a non-separating induced cycle of $G_1$, we have that $|C_{m+1}| \geq |C_2| \geq 5$.

**Claim 6.** *Every non-cut-vertex of $G_i - V(C_{m+1})$ contains at most one neighbor on $C_{m+1}$.*

*Proof.* Let $C' = C_{m+1} := u_0u_1 \dots u_{t-1}u_0$, where the indices are taken under the additive group $\mathbb{Z}_t$. By Lemma 4.4, every vertex of $\cup_{j\in[m]}C_j$ has at most one neighbor on $C_{m+1}$. Note that $|C_{m+1}| \geq 5$. By the minimality of $C_{m+1}$, every non-cut-vertex of $H_{m+1}$ has at most one neighbor on $C_{m+1}$. Suppose that a cut-vertex $b$ of $H_{m+1}$ is not a cut-vertex in $G_i - V(C_{m+1})$. Let $u_\alpha, u_\beta$ be two neighbors of $b$ on $C_{m+1}$. Let $F_1, \dots, F_n$ be all components of $G_i - V(C_{m+1}) - \{b\}$.

Suppose that $C'$ is odd, that is $t = 2h_o + 1$ for some $h_o \geq 2$. Let $Q'_e$ be the even path between $u_\alpha$ and $u_\beta$ in $C'$ and $2s$ denote the length of $Q'_e$. We may assume that $\beta = \alpha + 2s$. By Lemma 4.2, we have that $s \geq 2$ and at least one of $u_{\alpha+s-1}, u_{\alpha+s+1}$ has a neighbor $w \neq b$ in $H_{m+1}$. Without loss of generality, we may assume that $u_{\alpha+s-1}$ and $w$ are adjacent in $G$ and $w \in V(F_1)$. It follows that there exists $j_1 \in ([m] - i)$ such that $N_{F_1}(C_{j_1}) \neq \emptyset$ and $N_{H_{m+1}-F_1}(C_{j_1}) \neq \emptyset$. Let $C = C_{j_1} := v_0v_1 \dots v_{2l}v_0$, where the indices are taken under the additive group $\mathbb{Z}_{2\ell+1}$. Since $C_{j_1}$ is odd, by Lemma 4.1, we may assume that $v_0$ has a neighbor $z_1$ in $F_1$ and $v_\ell$ has a neighbor $z_2$ in $H_{m+1} - F_1$. Using the block structure, there exist two disjoint paths $L_1$ and $L_2$ such that $L_1$ links $z_1$ and $w$ in $H_{m+1}$ and $L_2$ links $z_2$ and $b$ in $H_{m+1}$. Then $C_{0,\ell} \cup v_0z_1 \cup L_1 \cup wu_{\alpha+s-1} \cup C'_{\alpha,\alpha+s-1} \cup u_\alpha b \cup L_2 \cup z_2v_\ell$, $C_{\ell,0} \cup v_0z_1 \cup L_1 \cup$

$wu_{\alpha+s-1} \cup C'_{\alpha,\alpha+s-1} \cup u_\alpha b \cup L_2 \cup z_2 v_\ell$, $C_{0,\ell} \cup v_0 z_1 \cup L_1 \cup wu_{\alpha+s-1} \cup C'_{\alpha+s-1,\beta} \cup u_\beta b \cup L_2 \cup z_2 v_\ell$, $C_{\ell,0} \cup v_0 z_1 \cup L_1 \cup wu_{\alpha+s-1} \cup C'_{\alpha+s-1,\beta} \cup u_\beta b \cup L_2 \cup z_2 v_\ell$ are 4 cycles of consecutive cycles. Therefore every non-cut-vertex of $G'_x$ has at most one neighbor on $C_{m+1}$.

Therefore $C'$ is even, that is $t = 2h_e$ for some $h_e \geq 3$. Suppose that $|\beta - \alpha| = 2$. Without loss of generality, we may assume that $\beta = \alpha + 2$. Since $G$ is $K_3$-free, $u_{\beta+1}$ has a neighbor $w_2 \neq b$ in $H_{m+1}$. Without loss of generality, we may assume that $w_2 \in V(F_1)$. It follows that there exists $j_2 \in ([m] - i)$ such that $N_{F_1}(C_{j_2}) \neq \emptyset$ and $N_{H_{m+1}-F_1}(C_{j_2}) \neq \emptyset$. Let $C = C_{j_2} := v_0 v_1 \dots v_{2l} v_0$, where the indices are taken under the additive group $\mathbb{Z}_{2\ell+1}$. Since $C_{j_2}$ is odd, by Lemma 4.1, we may assume that $v_0$ has a neighbor $z_1$ in $F_1$ and $v_\ell$ has a neighbor $z_2$ in $H_{m+1} - F_1$. Using the block structure, there exist two disjoint paths $N_1$ and $N_2$ such that $N_1$ links $z_1$ and $w_2$ in $H_{m+1}$ and $N_2$ links $z_2$ and $b$ in $H_{m+1}$. Then $C_{0,\ell} \cup v_0 z_1 \cup N_1 \cup u_{\beta+1} w_2 \cup C'_{\beta,\beta+1} \cup u_\beta b \cup N_2 \cup z_2 v_\ell$, $C_{\ell,0} \cup v_0 z_1 \cup N_1 \cup u_{\beta+1} w_2 \cup C'_{\beta,\beta+1} \cup u_\beta b \cup N_2 \cup z_2 v_\ell$, $C_{0,\ell} \cup v_0 z_1 \cup N_1 \cup u_{\beta+1} w_2 \cup C'_{\alpha,\beta+1} \cup u_\alpha b \cup N_2 \cup z_2 v_\ell$, $C_{\ell,0} \cup v_0 z_1 \cup N_1 \cup u_{\beta+1} w_2 \cup C'_{\alpha,\beta+1} \cup u_\alpha b \cup N_2 \cup z_2 v_\ell$ are 4 cycles of consecutive cycles. Therefore every two neighbors of $b$ on $C'$ are of distance more than 2 in $C'$.

Therefore, one of $u_{\alpha+h_e-1}, u_{\alpha+h_e+1}$ has a neighbor $w_3 \neq b$ in $H_{m+1}$. We may assume that $u_{\alpha+h_e-1}$ and $w_3$ are adjacent in $G$. Without loss of generality, we may assume that $w_3 \in V(F_1)$. It follows that there exists $j_3 \in ([m]-i)$ such that $N_{F_1}(C_{j_3}) \neq \emptyset$ and $N_{H_{m+1}-F_1}(C_{j_3}) \neq \emptyset$. Let $C = C_{j_3} := v_0 v_1 \dots v_{2l} v_0$, where the indices are taken under the additive group $\mathbb{Z}_{2\ell+1}$. Since $C_{j_3}$ is odd, by Lemma 4.1, we may assume that $v_0$ has a neighbor $z_1$ in $F_1$ and $v_\ell$ has a neighbor $z_2$ in $H_{m+1} - F_1$. Using the block structure, there exist two disjoint paths $M_1$ and $M_2$ such that $M_1$ links $z_1$ and $w_3$ in $H_{m+1}$ and $M_2$ links $z_2$ and $b$ in $H_{m+1}$. Then $C_{0,\ell} \cup v_0 z_1 \cup M_1 \cup w_3 u_{\alpha+h_e-1} \cup C'_{\alpha,\alpha+h_e-1} \cup b u_\alpha \cup M_2 \cup z_2 v_\ell$, $C_{\ell,0} \cup v_0 z_1 \cup M_1 \cup w_3 u_{\alpha+h_e-1} \cup C'_{\alpha,\alpha+h_e-1} \cup b u_\alpha \cup M_2 \cup z_2 v_\ell$, $C_{0,\ell} \cup v_0 z_1 \cup M_1 \cup w_3 u_{\alpha+h_e-1} \cup C'_{\alpha+h_e-1,\alpha} \cup b u_\alpha \cup M_2 \cup z_2 v_\ell$, $C_{\ell,0} \cup v_0 z_1 \cup M_1 \cup w_3 u_{\alpha+h_e-1} \cup C'_{\alpha+h_e-1,\alpha} \cup b u_\alpha \cup M_2 \cup z_2 v_\ell$ are 4 cycles of consecutive cycles.

Hence, $b$ contains at most one neighbor on $C_{m+1}$. This completes the proof of Claim 6. ∎

Now we may finish the proof of Theorem 1.2 as follows.

By Claims 5 and 6, $C_i, C_{m+1}, G - (V(C_i) \cup V(C_{m+1}))$ satisfy the conditions of Lemma 5.1 for any $i \in [m]$. Therefore there is no edges between $C_i$ and $C_{m+1}$, $G - (V(C_i) \cup V(C_{m+1}))$ is 2-connected and any vertex of $H_{m+1}$ has at most one neighbor in $\cup_{j\in[m+1]} V(C_j)$ in $G$.

We claim that $H_{m+1}$ is 2-connected. Let $C' = C_{m+1} := u_0 u_1 \dots u_{2h} u_0$, where the indices are taken under the additive group $\mathbb{Z}_{2h+1}$. Note that $\cup_{j\in[m]} C_j \cup H_{m+1}$ is 2-connected. Let $n$ be the minimum integer such that $H_{m+1} \cup (\cup_{j\leq n} C_j)$ is 2-connected but $D := H_{m+1} \cup (\cup_{j<n} C_j)$ is not 2-connected. Let $B_1, \dots, B_s$ be all end-blocks of $D$ with cut-vertices $b_1, \dots, b_s$ respectively. Note that $B_i$ is 2-connected for $i \in [s]$. Note that $C' \cup D$ is 2-connected, by Lemma 4.5, there exists an vertex $u_d$ on $C'$ such that for every $i \in [s]$, $N_{C'}(B_i - b_i) = \{u_d\}$ and there are 2 admissible paths $Q_{i,1}, Q_{i,2}$ between $u_d$ and $b_i$ in $B_i$ satisfying that $|E(Q_{i,1})| - |E(Q_{i,2})| = 1$. By the choice of $n$, we have that $D \cup C_n$ is 2-connected. Let $C = C_n := v_0 v_1 \dots v_{2l} v_0$, where the indices are taken under the additive group $\mathbb{Z}_{2\ell+1}$. By Lemma 4.5, there exists an vertex $v_f$ on $C$ such that for every $i \in [s]$, $N_C(B_i - b_i) = \{v_f\}$ and there are 2 admissible paths $P_{i,1}, P_{i,2}$ between $v_f$ and $b_i$ in $B_i$ satisfying that $|E(P_{i,1})| - |E(P_{i,2})| = 1$. Let $z_1$ be the neighbor of $u_{d+h}$ in $D$ and $z_2$ be the neighbor of $v_{f+\ell}$ in $D$. Since $v_{f+\ell}$ has at least two neighbors in $D$, we have that $z_1 \neq z_2$ and $z_1, z_2 \in D - (\cup_{j\in[s]} (B_j - b_j))$. Using the block structure, there exist $p, q$ such that there exist two disjoint paths $T_1, T_2$ such that $T_1$ links $z_1$ and $b_p$ and $T_2$ links $z_2$ and $b_q$ in $D - (\cup_{j\in[s]} (B_j - b_j))$. Then at least 4 of $C_{f,f+\ell} \cup P_{p,\alpha} \cup T_1 \cup z_1 u_{d+h} \cup C'_{d,d+h} \cup Q_{q,\beta} \cup T_2 \cup z_2 v_{f+\ell}$, $C_{f+\ell,f} \cup P_{p,\alpha} \cup T_1 \cup z_1 u_{d+h} \cup C'_{d,d+h} \cup Q_{q,\beta} \cup T_2 \cup z_2 v_{f+\ell}$, where $\alpha, \beta = 1, 2$ are consecutive cycles in $G$. Therefore $H_{m+1}$ is 2-connected.

Moreover, every vertex of $H_{m+1}$ has at most one neighbor in $\cup_{j\in[m+1]} V(C_j)$. It follows that $H_{m+1}$ has minimum degree at least 3. By Theorem 6.1, $H_{m+1}$ contains a non-separating induced cycle $C_{m+2}$ and let $H_{m+2} := H_{m+1} - V(C_{m+1})$. Since $G$ is finite, this process will terminate at a certain step and

we could find 3 desired cycles of consecutive lengths. This completes the proof of Theorem 1.2. ∎

## References


[1] J. Gao, Q. Huo, C. Liu and J. Ma, A unified proof of conjectures on cycle lengths in graphs, *Int. Math. Res. Not.*, to appear.

[2] J. Gao, Q. Huo and J. Ma, A strengthening on odd cycles in graphs of given chromatic number, *manuscript,* arXiv:

[3] U. Krusenstjerna-Hafstrøm and B.Toft, Special subdivisions of $K_4$ and 4-chromatic graphs, *Monatsh. Math.* **89** (1980), 101–110.

[4] C. Liu and J. Ma, Cycle lengths and minimum degree of graphs, *J. Combin. Theory Ser. B* **128** (2018), 66–95.

[5] C. Thomassen and B. Toft, Non-separating induced cycles in graphs, *J. Combin. Theory Ser. B* **31** (1981), 199–224.
